# Supplementary material for: AVS-Net: Audio-Visual Scale Net for Self-supervised Monocular Metric Depth Estimation
Source: arXiv:2412.01637 source file (2024-12-02)
Supplement: Supplementary file 1 [file X_suppl.tex]

\clearpage

\setcounter{page}{1}

\setcounter{section}{0}
\setcounter{figure}{0} 

\section{Supplementary materials}
\subsection{Performance with mean-std scaling}

\begin{table*}[!htb]
\caption{Quantitative results with mean/std scaling} 

\centering
\begin{tabular}{ccccccccc}
\hline Models & Scaling Method & $\mathbf{Abs\  rel}$ $\downarrow$ & $\mathbf{sq\  rel}$ $\downarrow$ & $\mathbf{R M S E} \downarrow$ & $\mathbf{R M S E}(\mathbf{l o g}) \downarrow$ & $\boldsymbol{\delta}_{\mathbf{1}} \uparrow$ & $\boldsymbol{\delta}_{\mathbf{2}} \uparrow$ & $\boldsymbol{\delta}_{\mathbf{3}} \uparrow$ \\
\hline \hline \multirow{3}{*}{ \makecell{Monodepth2}\cite{godard2019digging}} &  No  & 0.649 & 0.931& 1.656& 1.168& 0.008& 0.023& 0.065 	 \\
& RGB & 0.323 & 0.390& 1.054& 0.533& 0.388& 0.659& 0.821
	 \\ 
& RGB-Echo & 0.294 & 0.334& 0.921& 0.465& 0.495& 0.756& 0.876

 	 \\
\cmidrule(r){2-9}
\multirow{2}{*}{ \makecell{MonoVit}\cite{zhao2022monovit}} & No   & 0.568 & 0.757& 1.490& 0.998& 0.017& 0.072& 0.283 	 \\ 
& RGB & 0.314 & 0.368& 1.038& 0.550& 0.397& 0.673& 0.825
 	 \\
& RGB-Echo & 0.284 & 0.307& 0.900& 0.499& 0.509& 0.764& 0.877

	 \\
 \cmidrule(r){2-9}
\multirow{2}{*}{ \makecell{LiteMono}\cite{zhang2023lite}}  & No    & 0.782 & 1.284& 1.933& 1.626& 0.000& 0.000& 0.001\\ 
 & RGB & 0.314 & 0.375& 1.055& 0.528& 0.402& 0.669& 0.822 \\
& RGB-Echo  & 0.287 & 0.321& 0.927& 0.471& 0.502& 0.757& 0.877

	 \\
\hline

\multirow{3}{*}{ \makecell{ZoeDepth}\cite{bhat2023zoedepth}}  & No(zero-shot)  & 1.000 & 1.630& 1.558& 0.705& 0.107& 0.258& 0.486 \\ 
& RGB & 0.310 & 0.348& 1.007& 0.626& 0.418& 0.682& 0.823

\\ 
& RGB-Echo  & 0.278 & 0.278& 0.859& 0.515& 0.521& 0.765& 0.872

\\ 

 \cmidrule(r){2-9}
\multirow{3}{*}{ \makecell{Jun et al.,}\cite{jun2022depth}}  & No(zero-shot)  & 0.549 & 0.597& 1.083& 0.483& 0.241& 0.532& 0.828 \\ 

& RGB & 0.331 & 0.373& 1.050& 0.853& 0.411& 0.659& 0.791
\\ 

& RGB-Echo & 0.319 & 0.326& 0.928& 0.854& 0.472& 0.721& 0.833
 \\ 

\cmidrule(r){2-9}

\multirow{3}{*}{ \makecell{NeWCRFs \cite{yuan2022neural}}}  & No(zero-shot)  & 1.240 & 2.485& 1.874& 0.813& 0.094& 0.208& 0.388 \\ 

& RGB & 0.332 & 0.382& 1.054& 0.790& 0.402& 0.654& 0.794
 \\ 

& RGB-Echo & 0.320 & 0.326& 0.921& 0.745& 0.461& 0.722& 0.843
\\ 

\hline
\hline

\end{tabular}

\label{tab:MeanStdAblation}
\end{table*}

\subsection{Training details}
\subsubsection{AVS-Net training details}

For the AVS-Net and the corresponding only-RGB baseline (ZoeDepth), we keep the pre-trained Midas encoder-decoder frozen, with other parts trainable, with the objective of keeping the quality of relative depth model weight trained across 12 datasets. Both AVS-Net(RGB-Echo) and AVS-Net(Only-RGB) were trained for 80 epochs with early stopping and a patience value of 20 epochs. OneCycleLR schedular \cite{smith2019super} with initial learning rate $1.6\times10^{-4}$ and batch size $2$ are used. The best model weights with lowest ABS Rel were saved and used for final evaluations. 

\subsubsection{self-supervised depth models training details}
Following \cite{godard2019digging,zhao2022monovit,zhang2023lite} the per-pixel binary auto masking strategy $\mu$ is applied to tackle stationary scene or objects moving with cameras. The experiments were conducted based on Monodepth2 \cite{godard2019digging}, MonoVit \cite{zhao2022monovit} and Lite-Mono \cite{zhang2023lite}, with an initial learning rate of $1e-4$, a batch size of 12 and training conducted for 20 epochs. For the weight initialization, the depth encoder for Monodepth2 is initialised with ImageNet \cite{russakovsky2015imagenet} pre-trained weights, the depth encoder and decoder for MonoVit is from ImageNet-1K \cite{russakovsky2015imagenet} pretrained MPViT-small weight. For Lite-Mono, we used standard lite-mono architecture with intermediate channel numbers $[48, 80, 128]$, following official implementation, kaiming initialization \cite{he2015delving} is used for convolutional layers, with 0-1 initialization for Layer Normalization and Batch Normalization layers.

\subsection{Zero-shot metric depth model details} For the pre-trained weights for zero-shot metric depth models, ZoeDepth is load from Zoe-D-NK \cite{bhat2023zoedepth} weight, which is trained on 12 relative depth datasets, fintuned on both NYUv2 \cite{silberman2012indoor} and KITTI\cite{geiger2012we}. NeWCRFs\cite{yuan2022neural} is trained on NYUv2 dataset. Jun et al.,\cite{jun2022depth} is trained on both NYUv2 and HR-WSI \cite{xian2020structure} datasets. 

\subsection{Considerations for BatVision dataset split}
As $BV2$ covers larger variety in terms of scene types (both indoor and outdoor) and depth ranges (0-30m) than $BV1$ (0-12m).
